# Supplementary material for: Ab initio Leading Order Effective Potentials for Elastic Nucleon-Nucleus Scattering
Source: arXiv:2005.00111 ancillary file (2020-04-30)
Supplement: Supplementary file 1 [file SupplementalMaterials.pdf]

# ***Ab initio* Leading Order Effective Potentials for Elastic Nucleon-Nucleus Scattering Supplemental Materials**

M. Burrows<sup>(a)</sup>, R. Baker<sup>(a)</sup>, Ch. Elster<sup>(a)</sup>, S.P. Weppner<sup>(b)</sup>, K.D. Launey<sup>(c)</sup>, P. Maris<sup>(d)</sup>, and G. Popa<sup>(a)</sup>

*(a) Institute of Nuclear and Particle Physics,  
and Department of Physics and Astronomy,  
Ohio University, Athens, OH 45701, USA*

*(b) Natural Sciences, Eckerd College,  
St. Petersburg, FL 33711, USA*

*(c) Department of Physics and Astronomy,  
Louisiana State University,  
Baton Rouge, LA 70803, USA*

*(d) Department of Physics and Astronomy,  
Iowa State University, Ames, IA 50011, USA*

(Dated: April 30, 2020)

PACS numbers: 24.10.-i, 24.10.Ht, 25.40.-h, 25.40.Cm

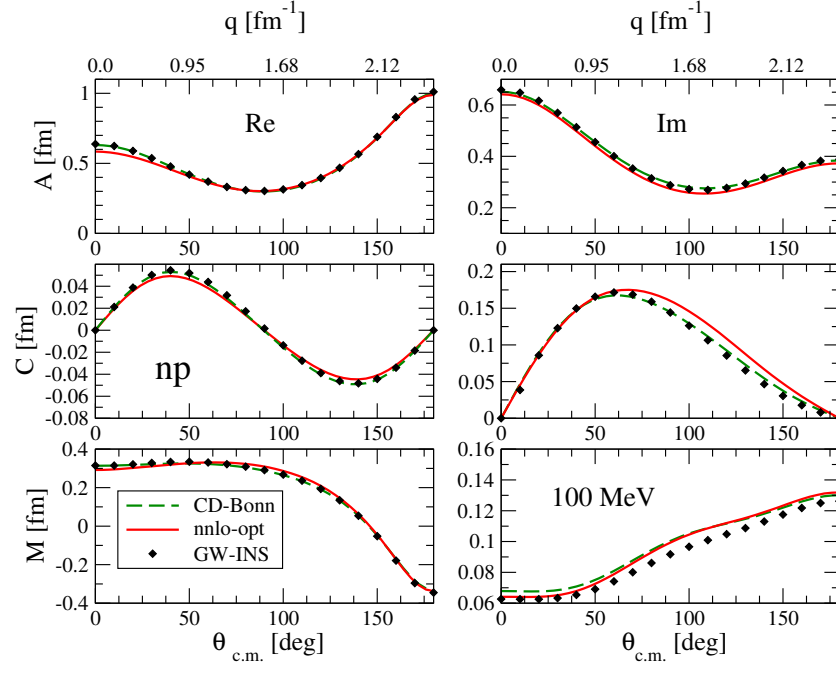

FIG. 1. Wolfenstein amplitudes  $A$  and  $C$  as function of the scattering angle and momentum transfer for  $np$  scattering at 100 MeV laboratory kinetic energy. The solid (red) line represents the  $\text{NNLO}_{\text{opt}}$  chiral interaction [1], and the dashed (green) line the CD-Bonn potential [2]. The solid diamonds stand for the extraction from the GW-INS analysis [3].

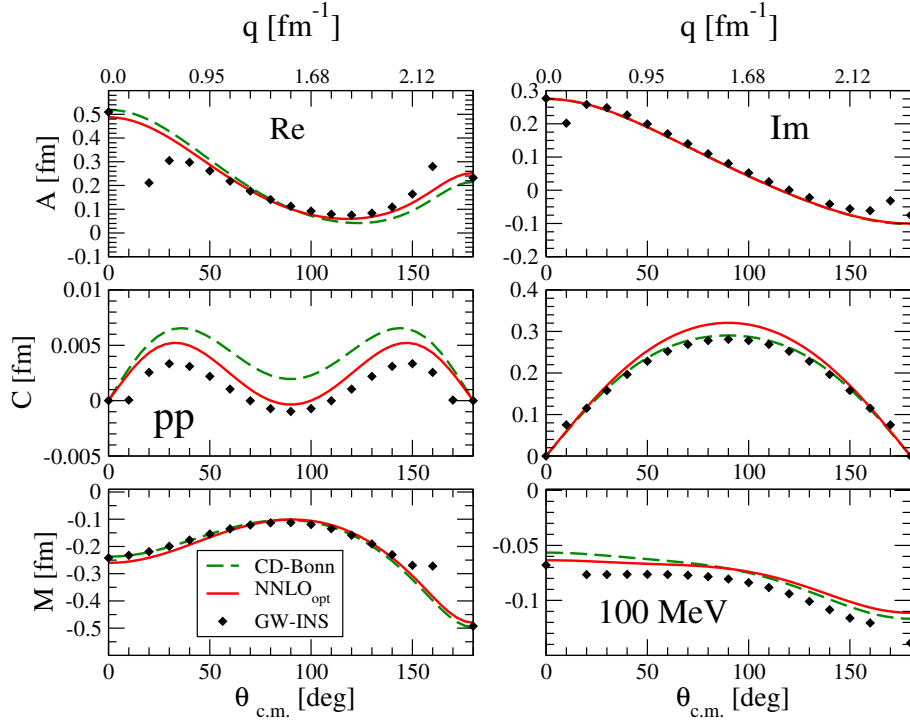

FIG. 2. Same as Fig. 1 for  $pp$  scattering at 100 MeV laboratory kinetic energy.

- 
- [1] A. Ekström, G. Baardsen, C. Forssén, G. Hagen, M. Hjorth-Jensen, G. R. Jansen, R. Machleidt, W. Nazarewicz, *et al.*, Phys. Rev. Lett. **110**, 192502 (2013).
  - [2] R. Machleidt, Phys. Rev. **C63**, 024001 (2001), arXiv:nucl-th/0006014.
  - [3] R. L. Workman, W. J. Briscoe, and I. I. Strakovsky, Phys. Rev. **C94**, 065203 (2016), arXiv:1609.01741 [nucl-th].
